# Supplementary material for: Effective operators in $t$-channel single top production and decay
Source: arXiv:1807.03576 source file (2018-07-10)

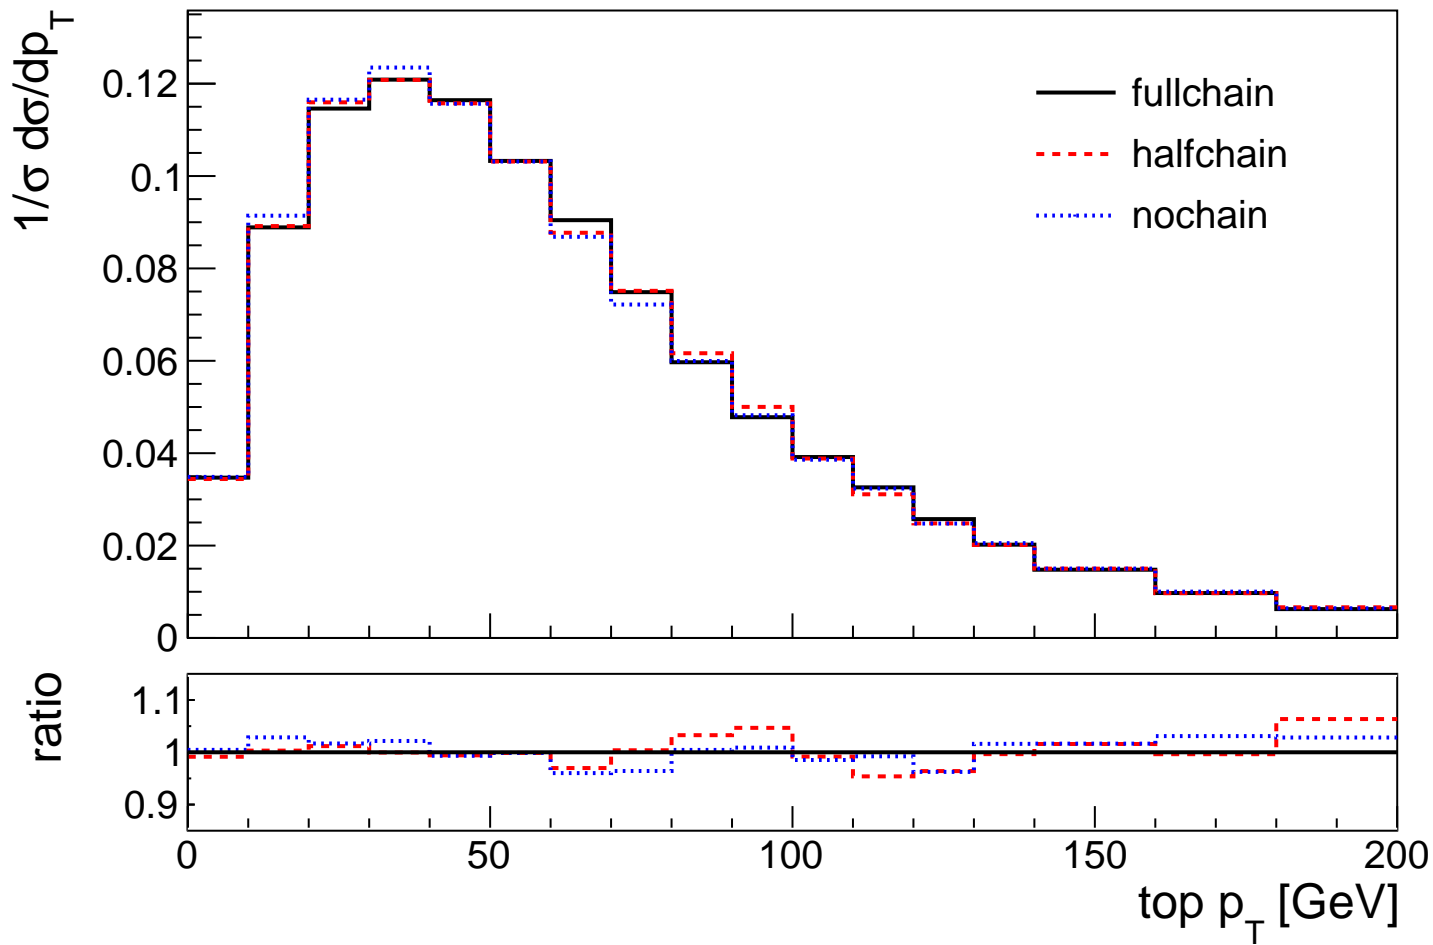

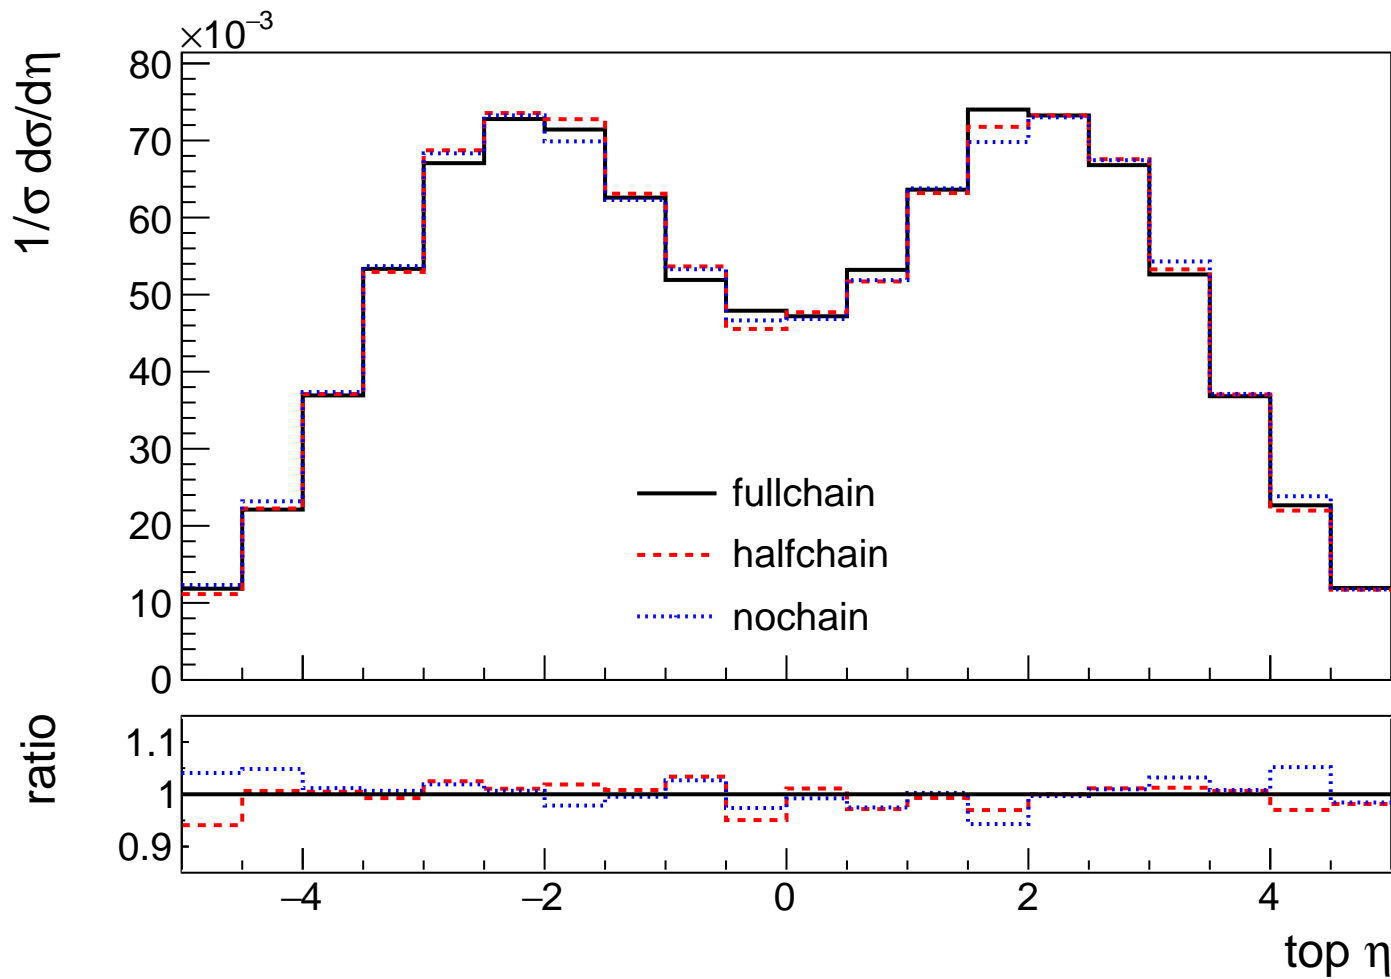

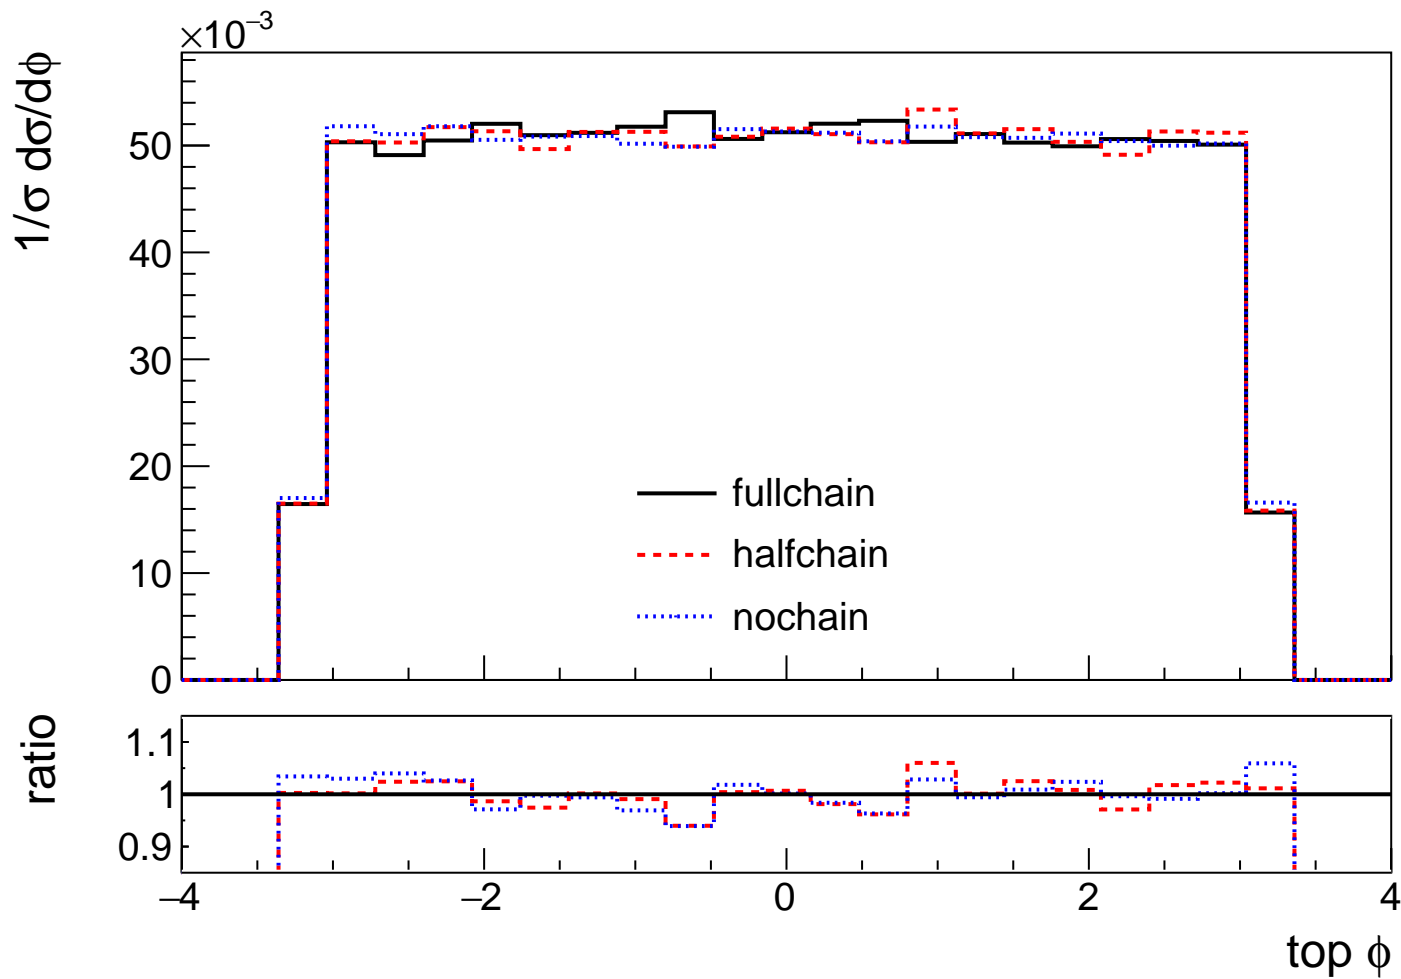

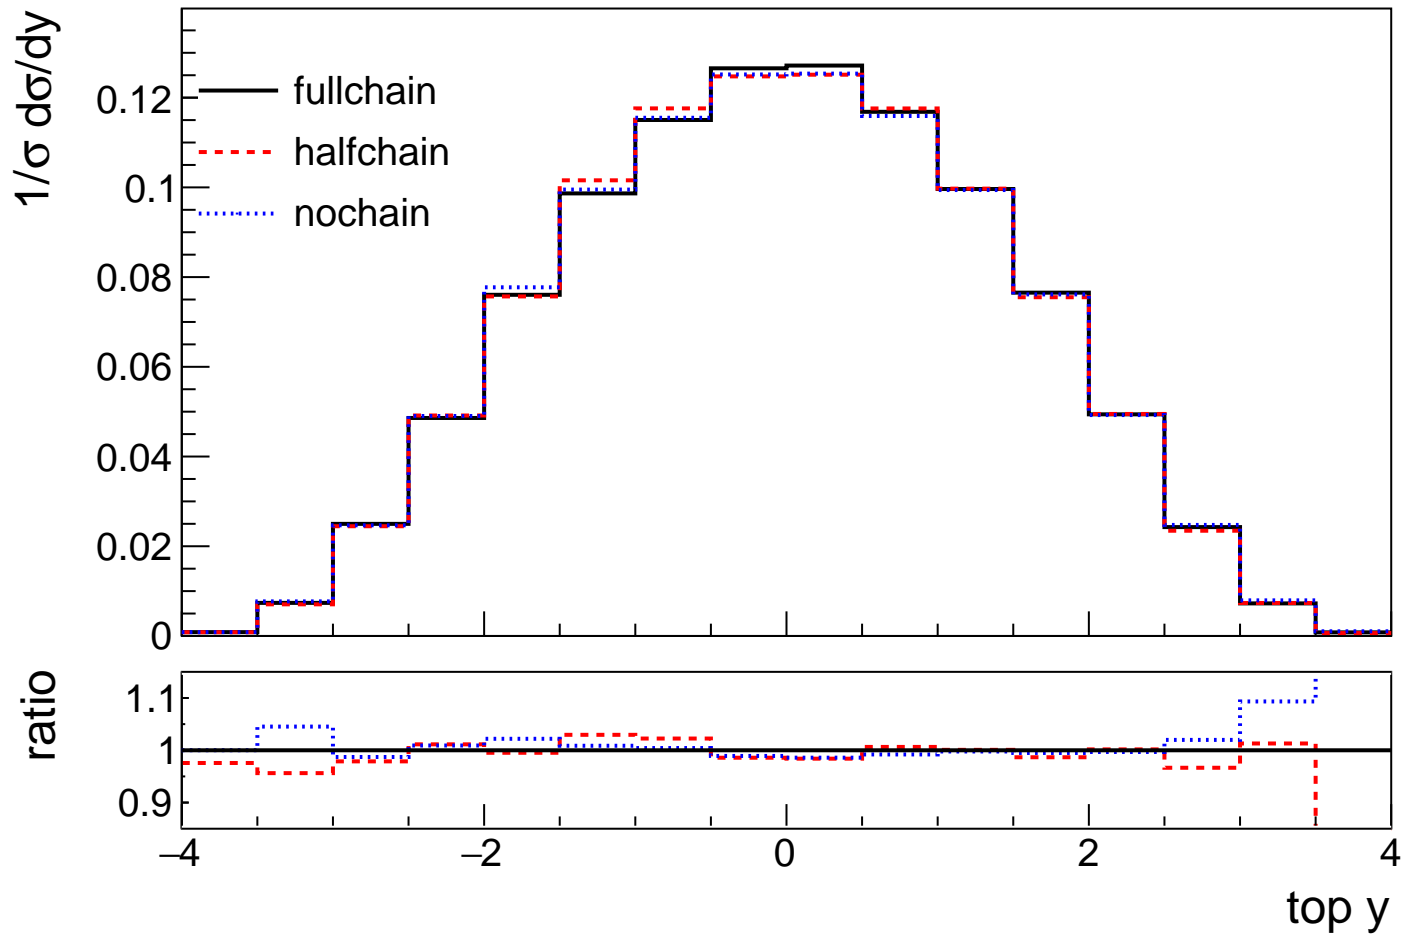

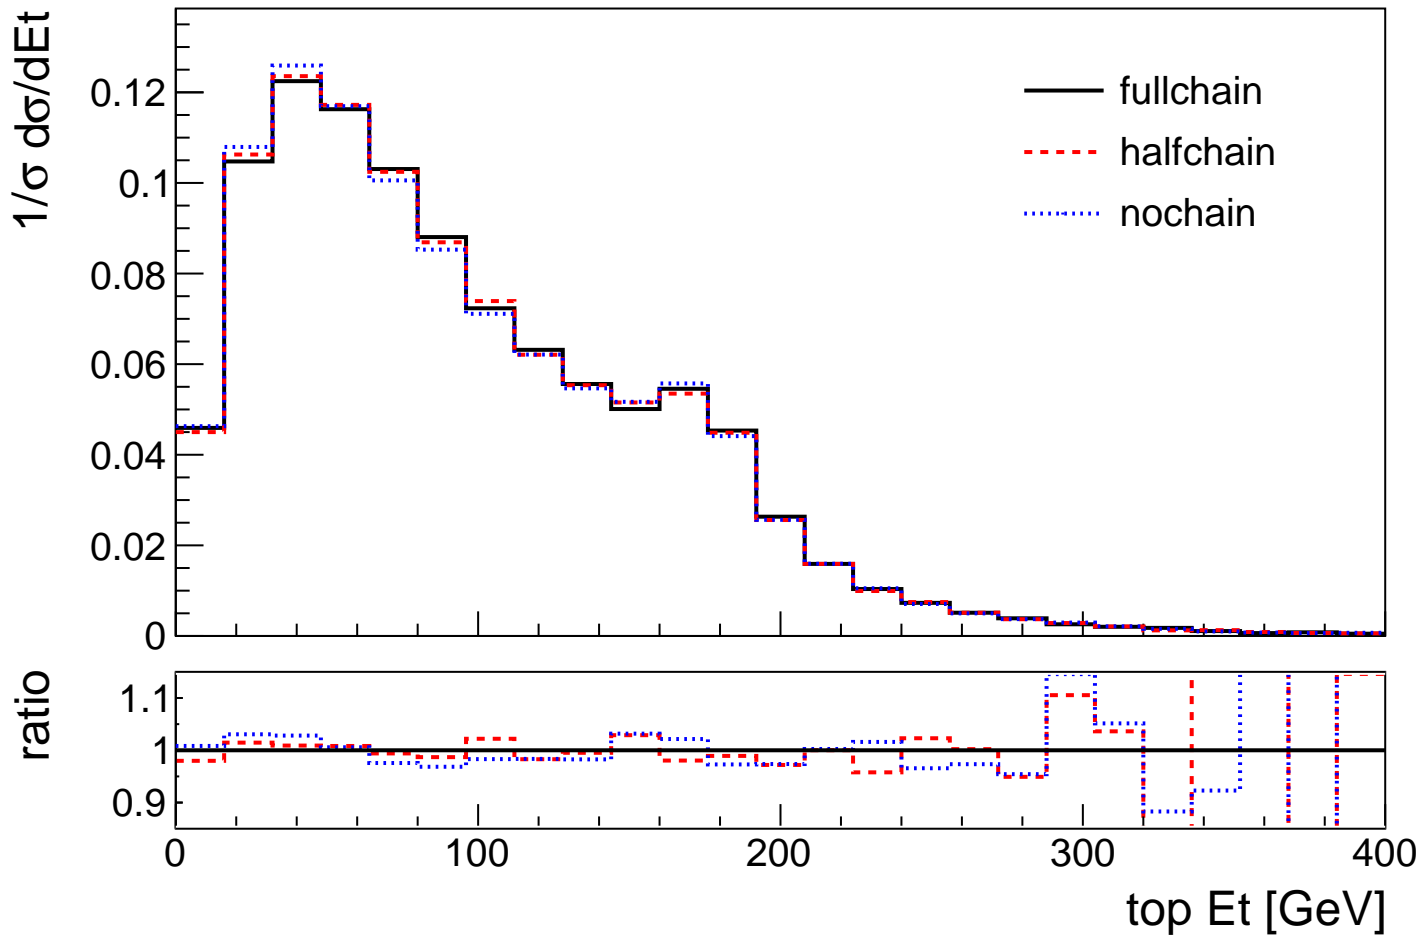

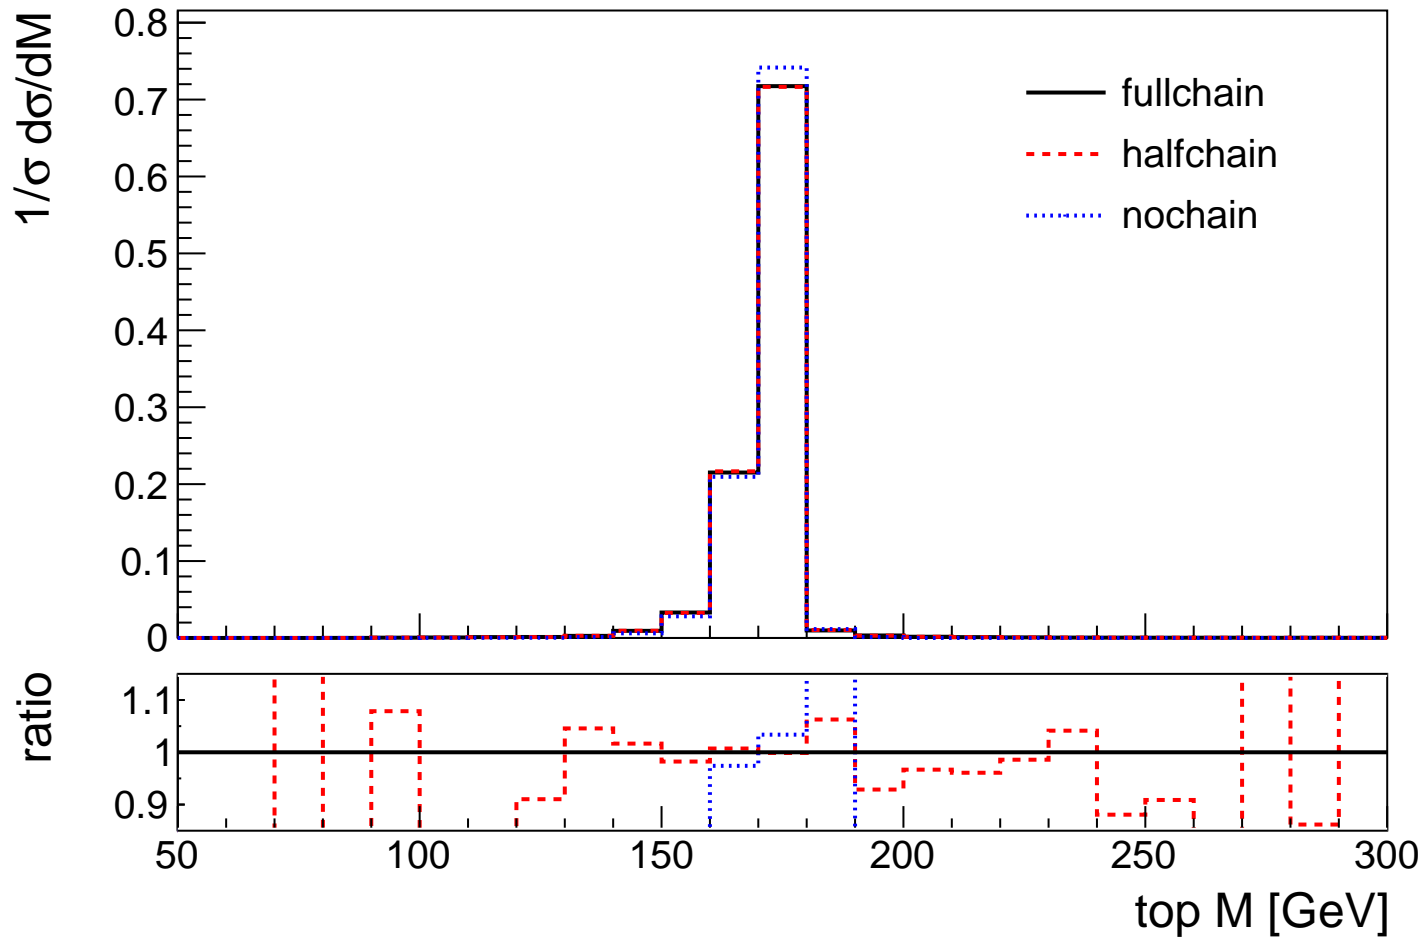

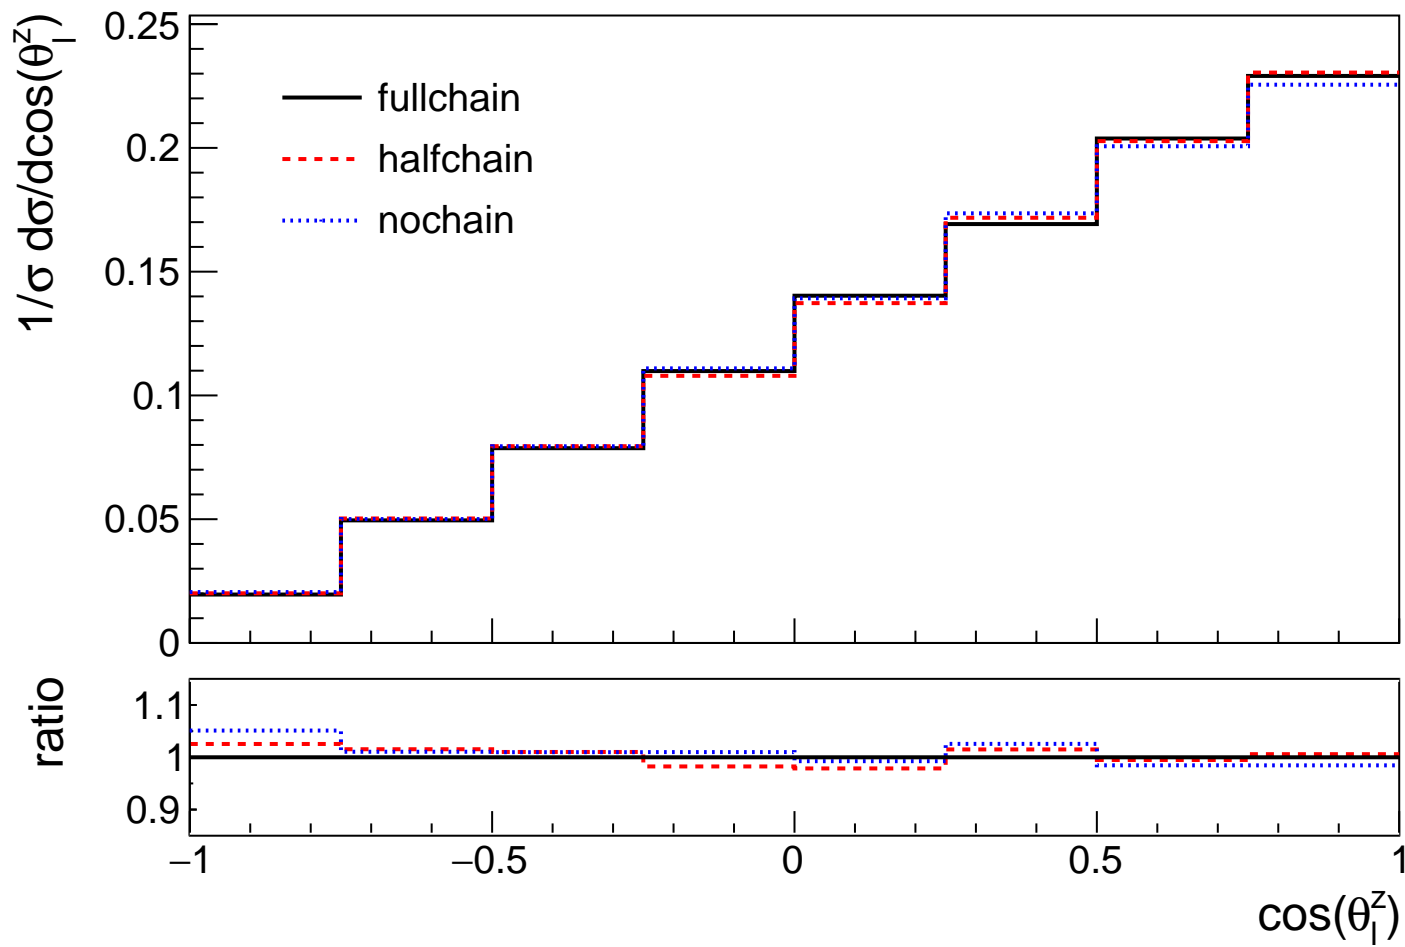

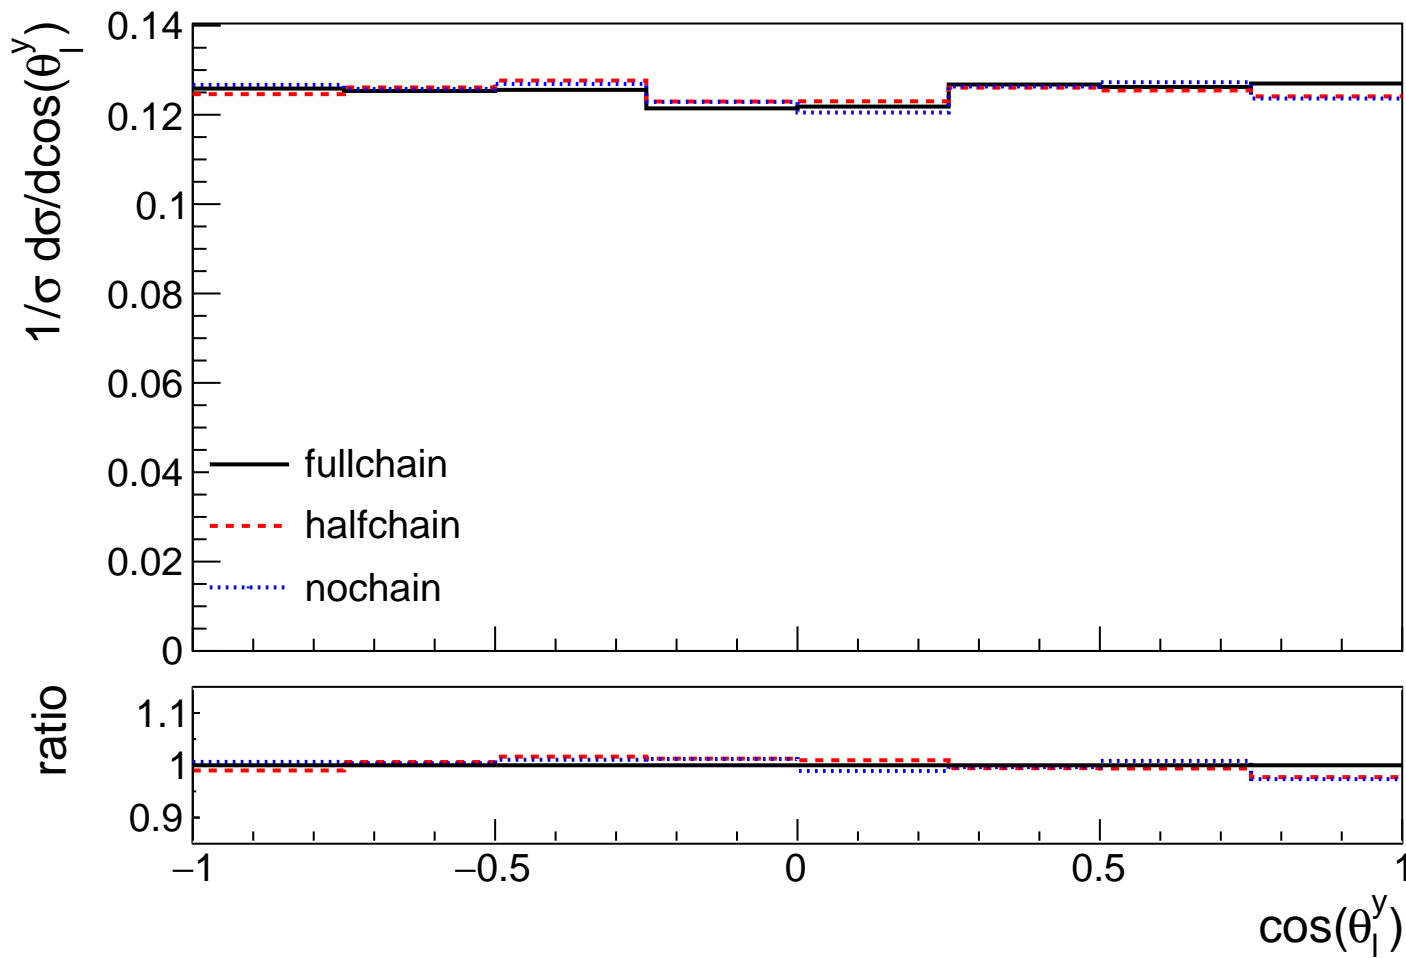



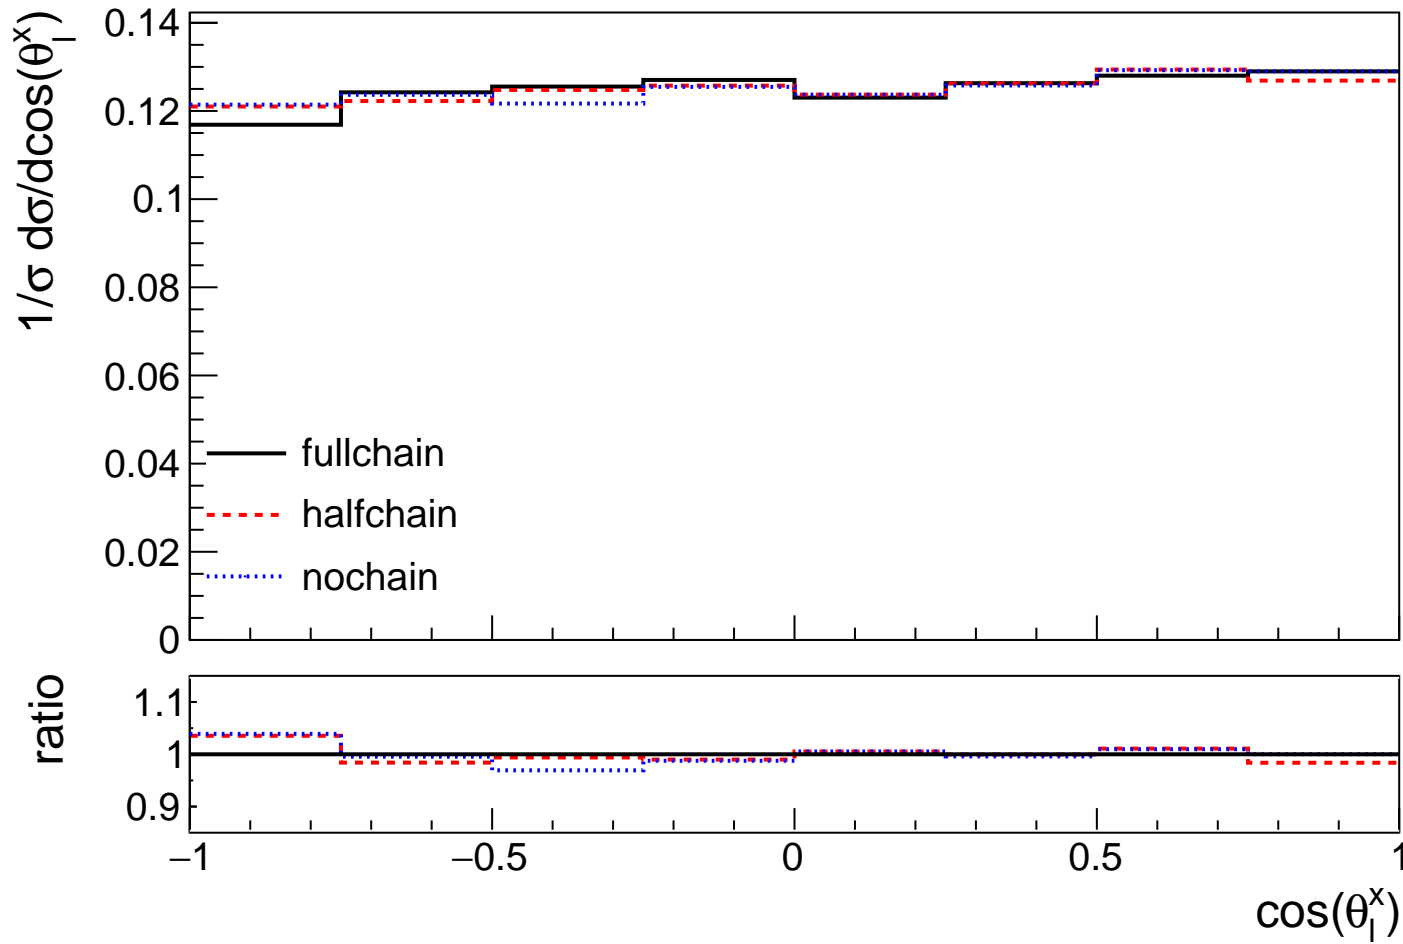

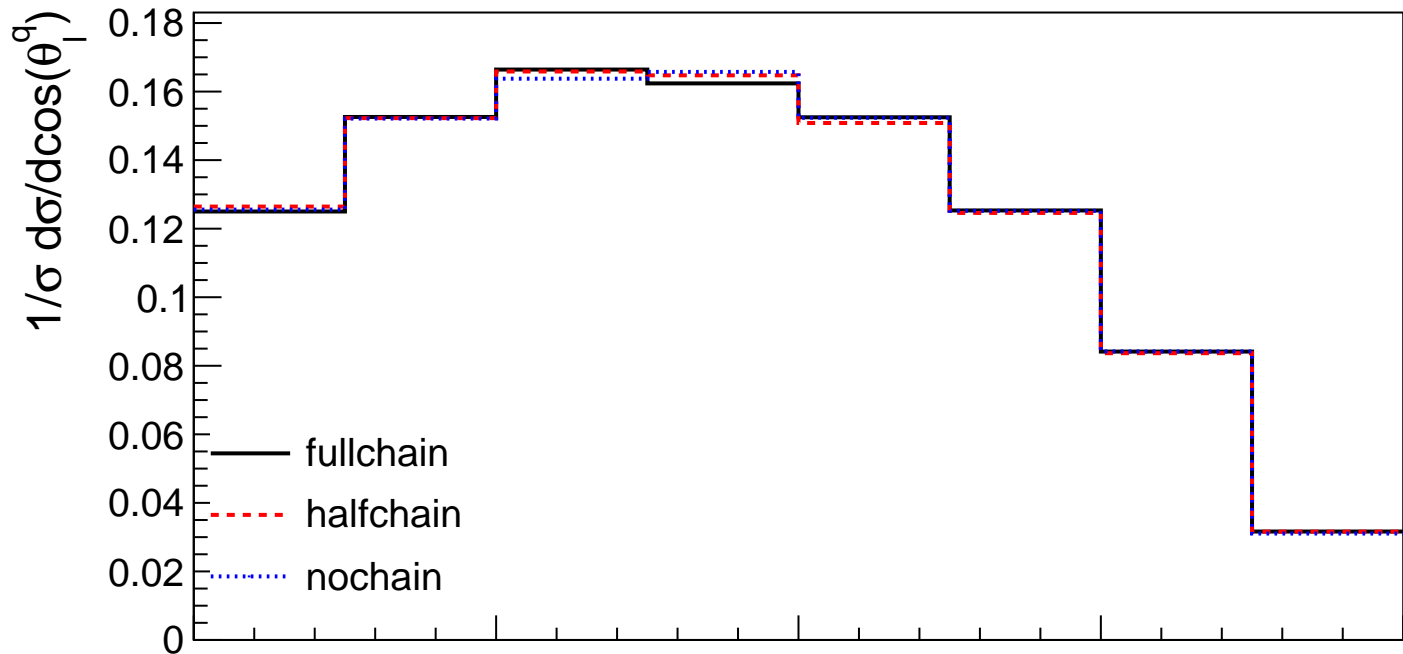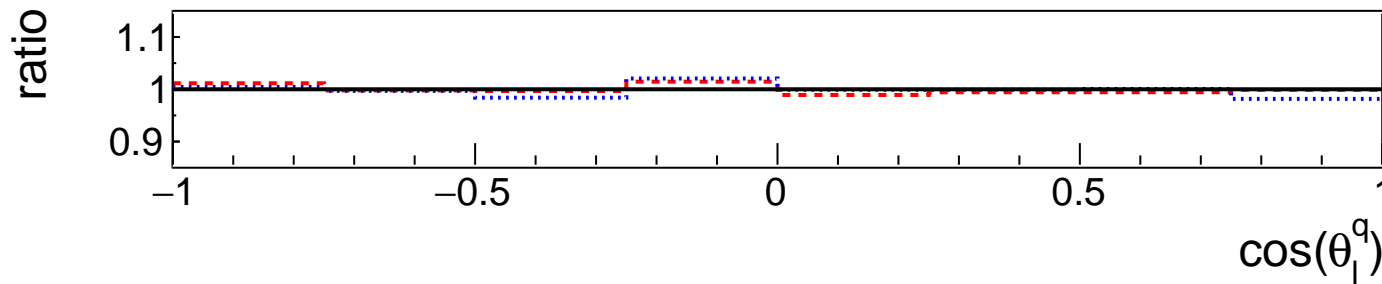

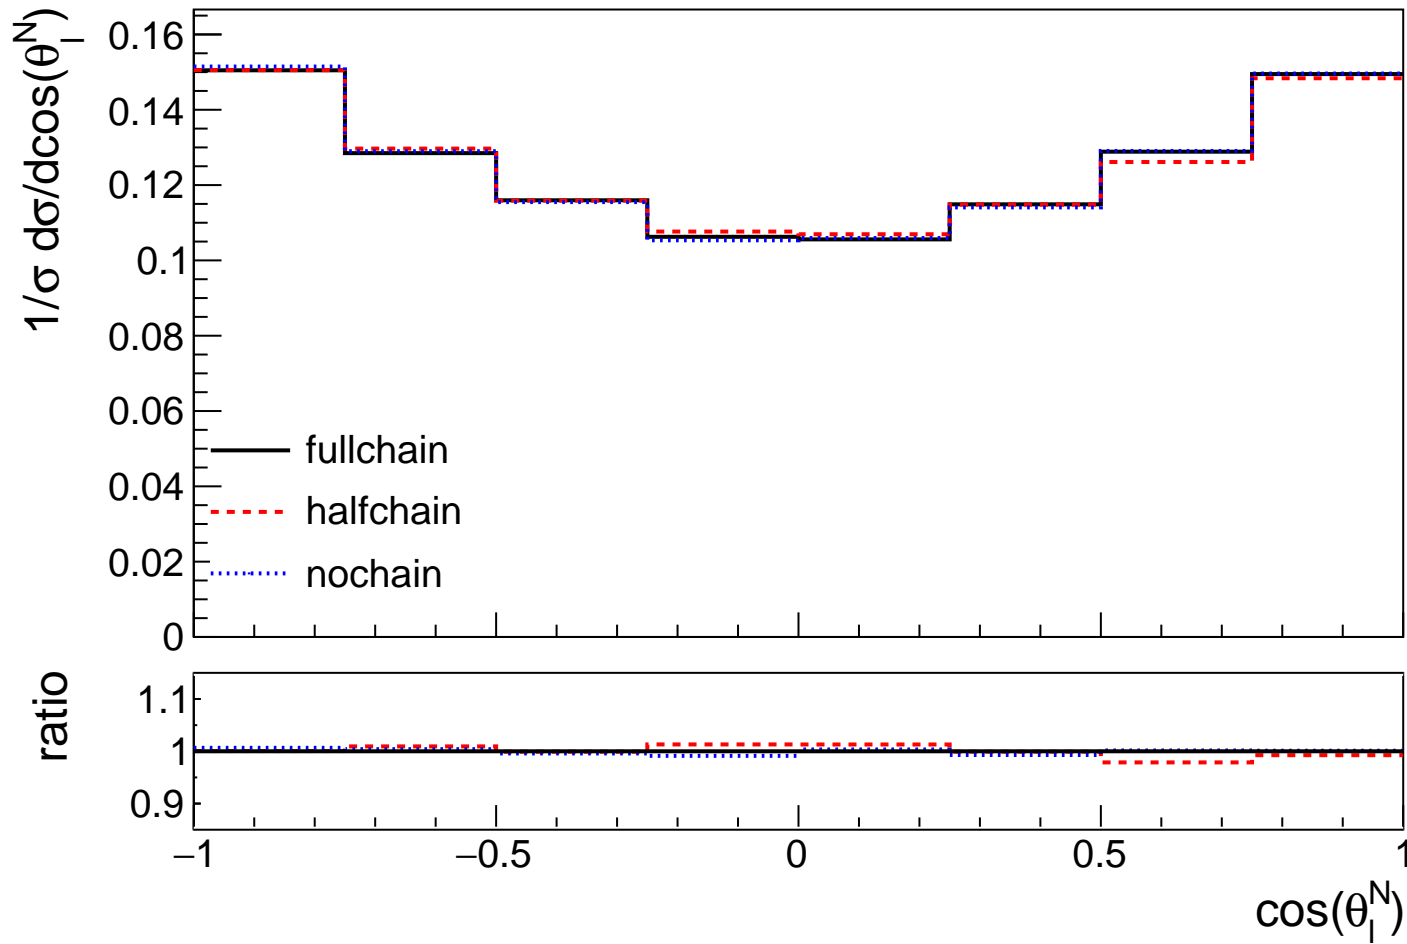

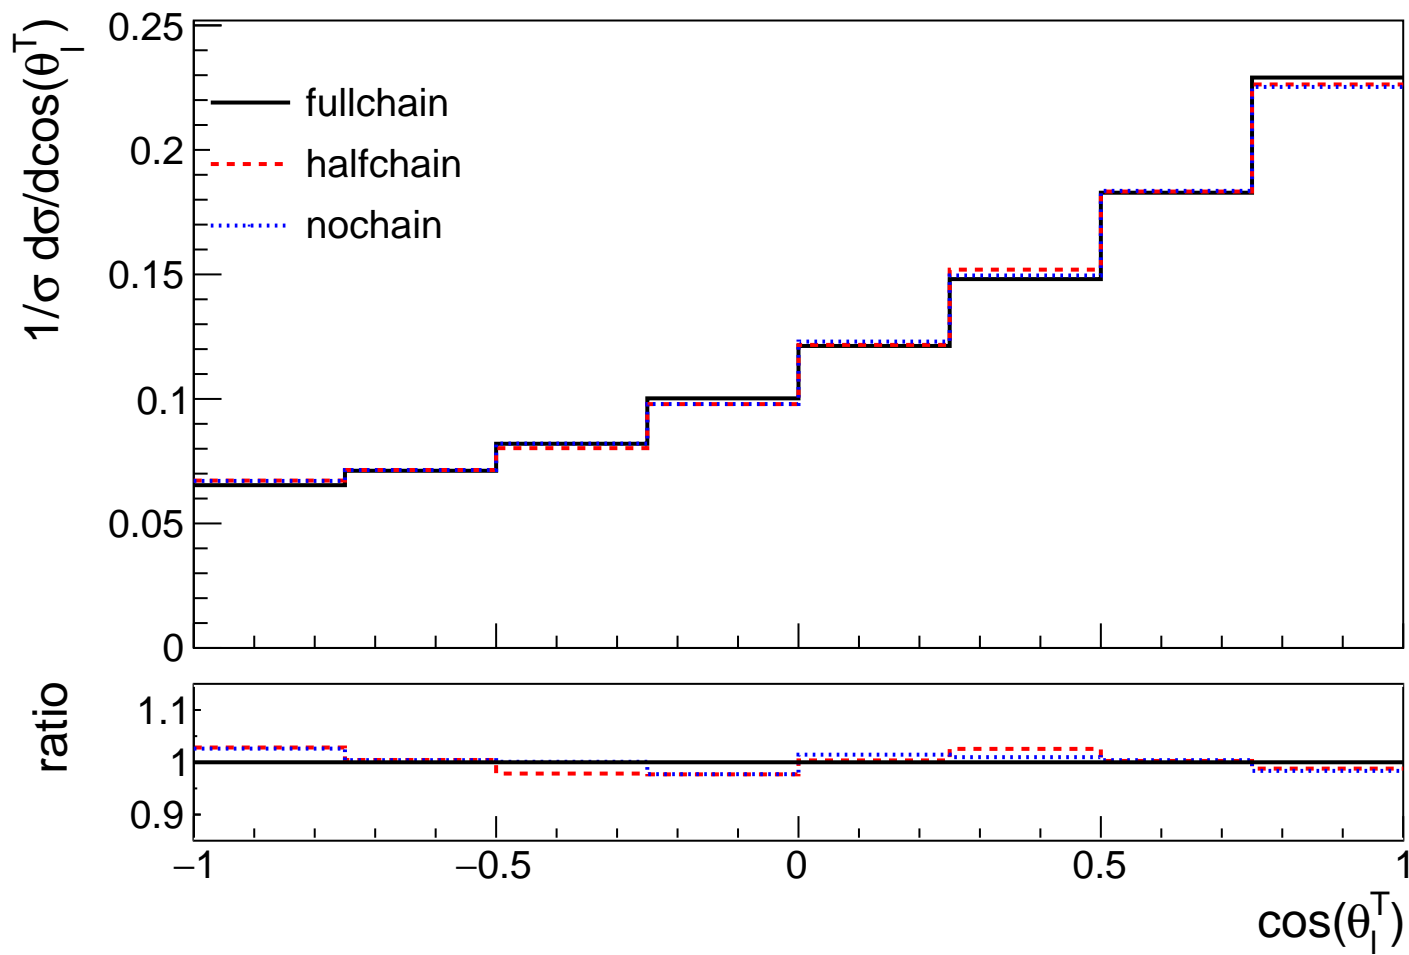

Supplement: Supplementary file 1 [file SM_LO_chain_analysis.pdf]
